# Supplementary material for: MoE-Infinity: Efficient MoE Inference on Personal Machines with Sparsity-Aware Expert Cache
Source: arXiv:2401.14361 source file (2025-03-12)
Supplement: Supplementary file 1 [file appendix-evaluation.tex]

\section{Evaluation of \sys in Serving}
\label{sec:eval-serving}

\mypar{Hardware} We show our experimental results on a commodity 8-GPU server which has eight NVIDIA RTX A5000 GPUs and 1TB of DRAM host memory. These GPUs are connected in pair-wise NVLink, and each GPU is connected to the host memory through a dedicated PCIe 4.0 connection (32GB/s). 
To demonstrate both GPU-poor and GPU-rich cases, we scale the resource from using only 1 GPU (for GPU-poor) to 8 GPUs (for GPU-rich).
Unless otherwise mentioned, \sys is evaluated using a single GPU.

\begin{figure*}[t]
    \centering
    \begin{minipage}{\linewidth}
        \centering
        \includegraphics[width=.85\linewidth]{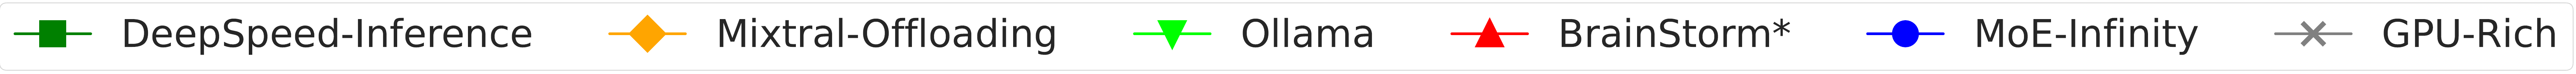}
    \end{minipage}
    % \newline
    \begin{minipage}{.24\linewidth}
        \centering
        \includegraphics[width=\linewidth]{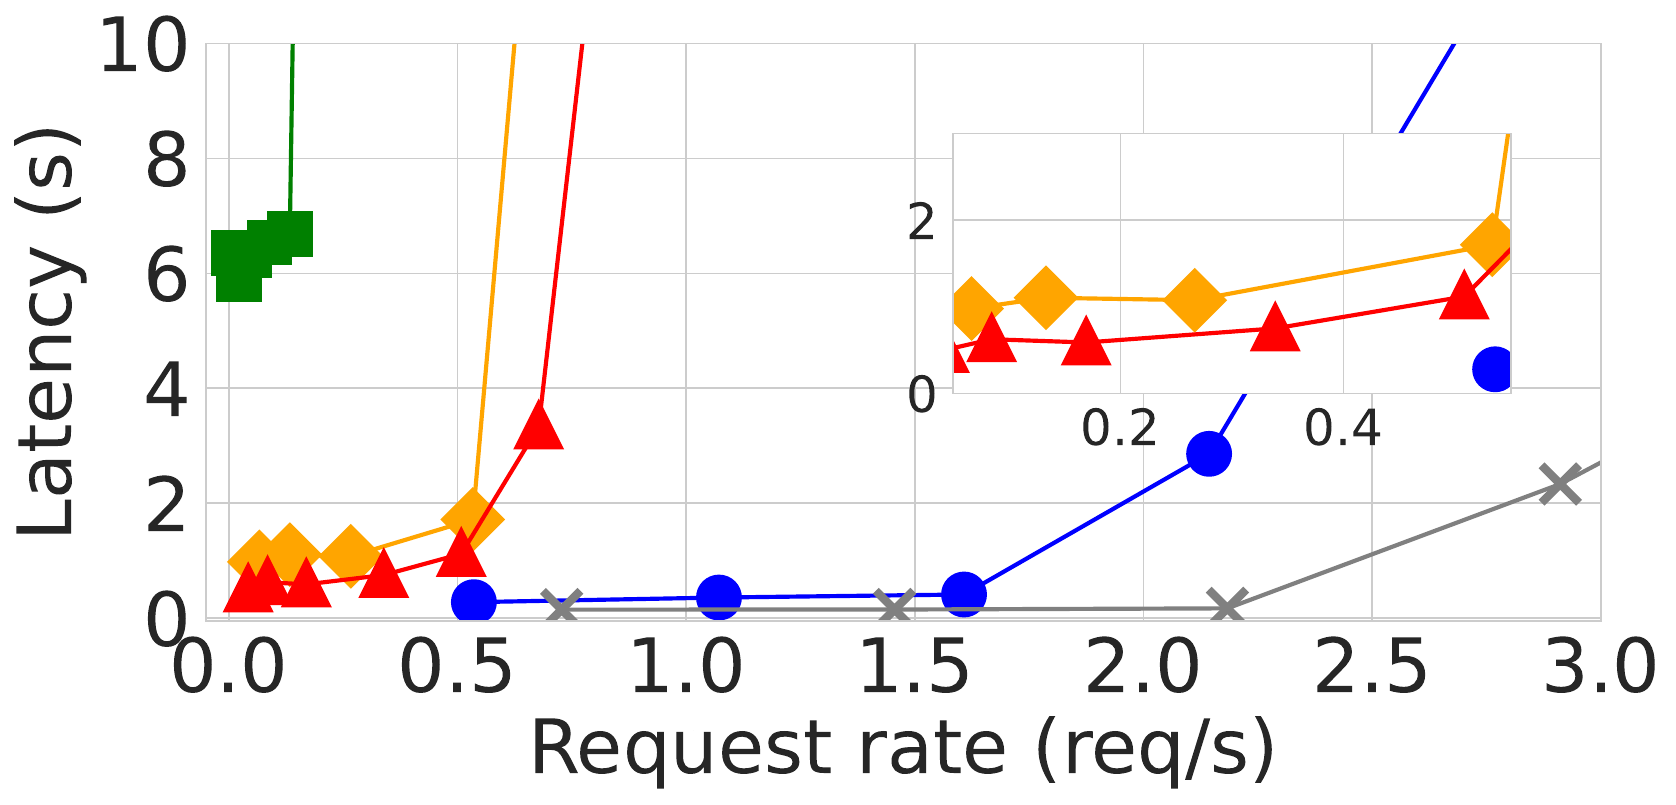}
        % \caption{Switch-128x0.2B}
        \label{fig:rps-latency-switch}
    \end{minipage}
    \begin{minipage}{.24\linewidth}
        \centering
        \includegraphics[width=\linewidth]{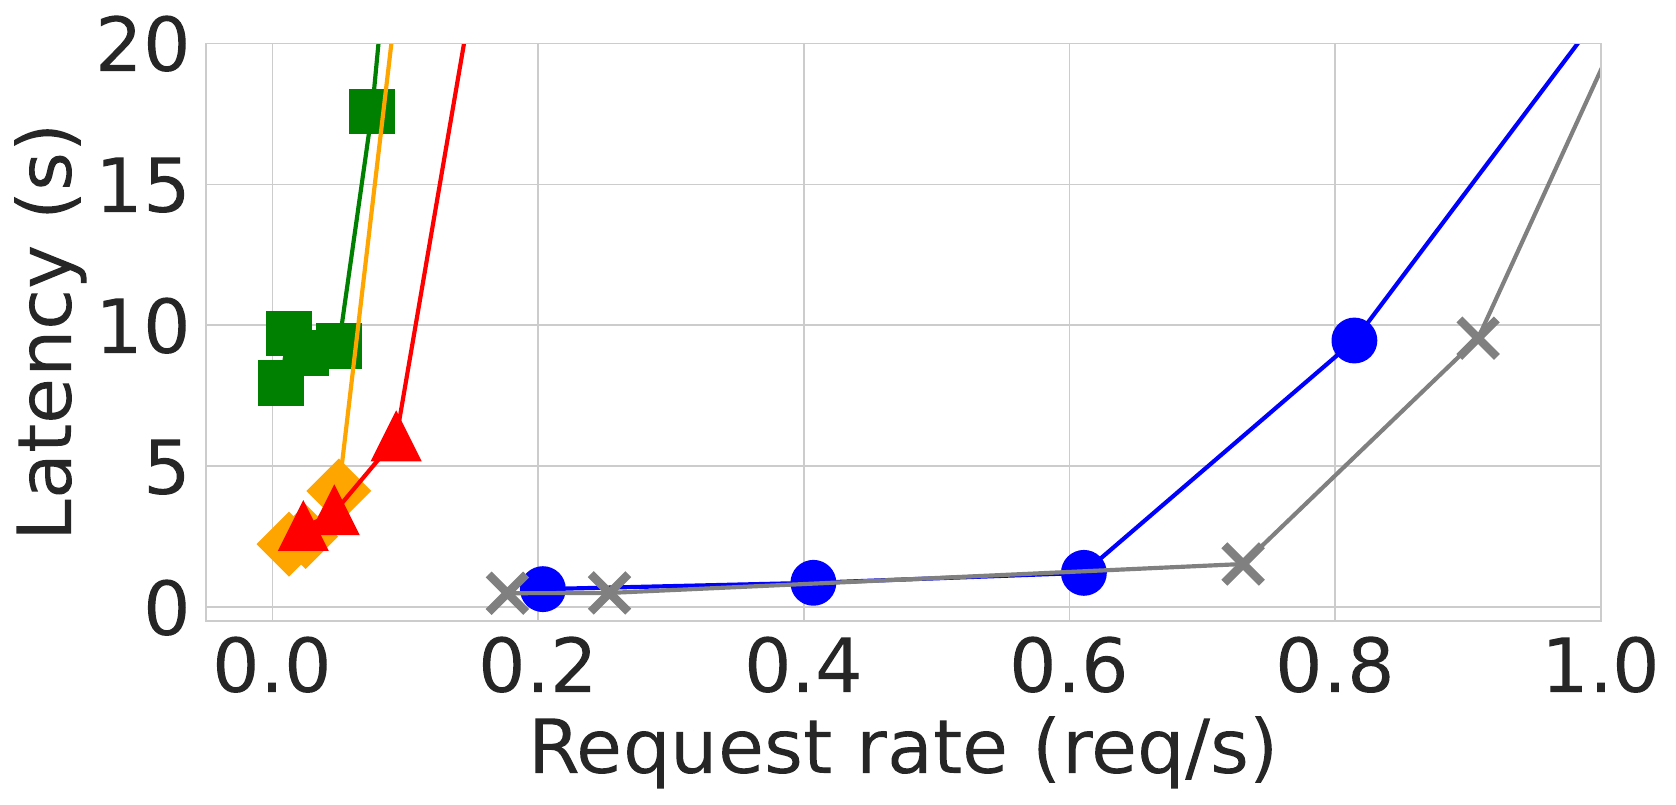}
        % \caption{NLLB-128x0.4B}
        \label{fig:rps-latency-nllb}
    \end{minipage}
    \begin{minipage}{.24\linewidth}
        \centering
        \includegraphics[width=\linewidth]{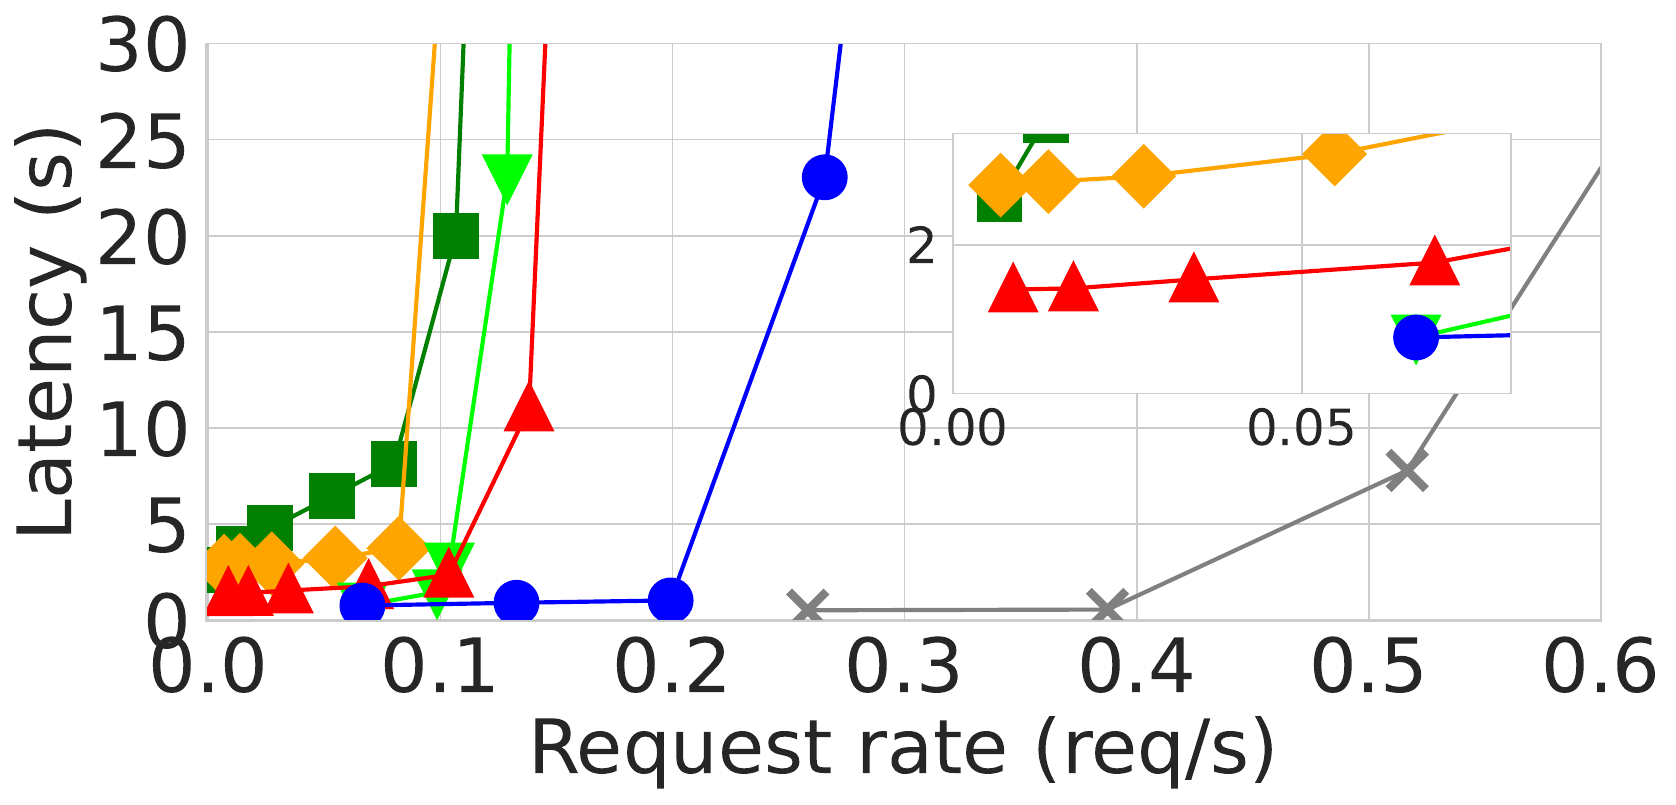}
        % \caption{Mixtral-8x7B}
        \label{fig:rps-latency-mixtral}
    \end{minipage}
    \begin{minipage}{.24\linewidth}
        \centering
        \includegraphics[width=\linewidth]{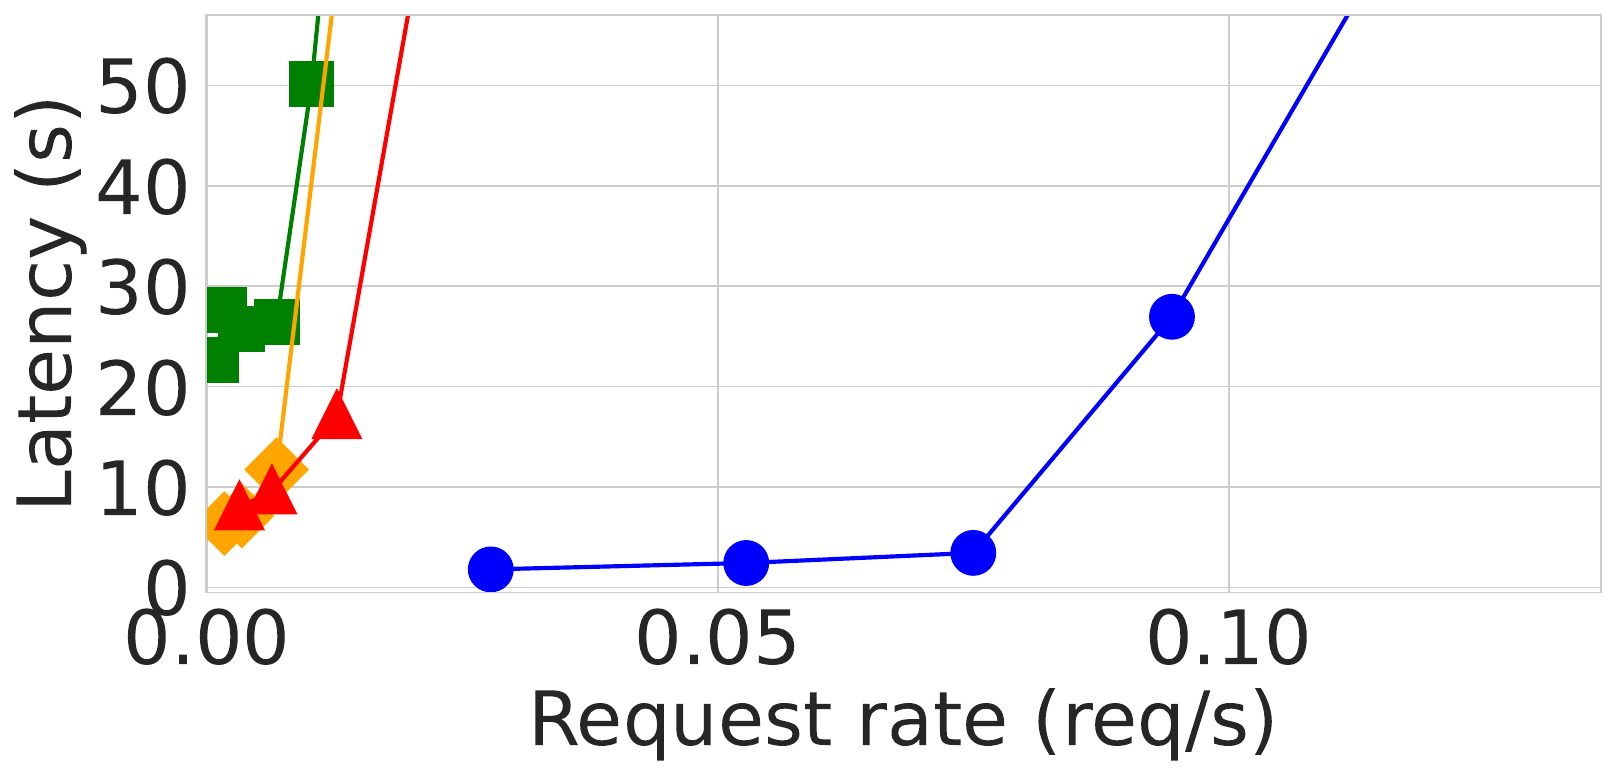}
        % \caption{Arctic-128x4B}
        \label{fig:rps-latency-arctic}
    \end{minipage}
    \hfill
    \vspace{-0.15in}
    \begin{minipage}{\linewidth}
        \centering
        \includegraphics[trim={0 4in 0 0},clip,width=\linewidth]{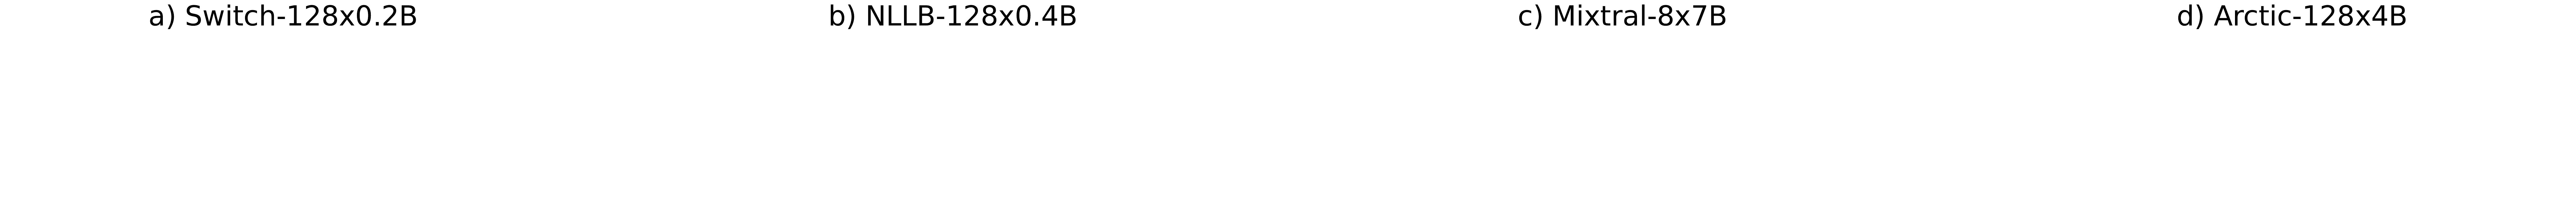}
    \end{minipage}
    \caption{End-to-end performance. For Switch and Mixtral, the sub-figures detail the sub-second latency.GPU-rich is omitted for Arctic since this model cannot be fully fitted to GPUs on a single server.}
    \label{fig:rps-latency}
\end{figure*}

\mypar{Serving dataset}
To emulate a real-world LLM serving workload, we implement inference clients which send their requests with intervals following the distribution modelled after Azure Trace~\cite{azuretrace}.  Without further mention, these clients uniformly select the prompts from all LLM tasks in three datasets by default, emulating a generic ChatBot service. This workload approach follows recent leading LLM serving studies~\cite{vllm, phantom}.

\subsection{Entire \sys in Action}

We now assess the performance and benefits when putting entries \sys in action for serving MoE models. In addition to the baseline systems mentioned above, we consider one more baseline, named \emph{GPU-Rich}, which represents the users with affluent GPU resources and can deploy the entire MoE models to a larger number of GPUs. This GPU-Rich baseline can show the best latency and throughput performance and inform us the performance cost of \sys. 

% Baselines:
% - DeepSpeed-Inference - support MoE offloading and comparable performance with vLLM, represent dependency next-layer prefetching + LRU for caching 
% - Mixtral Offloading - on-demand + LRU
% - Llama.cpp - cache + swap??????
% - BraintStorm - not open-sourced implemented correlation analysis within Archer, representing the correlation analysis for preftehcing and caching
% - Ideal - Archer performance with GPU onlys. The ideal case for Archer without any offloading costs. 

\mypar{End-to-end performance} We report the end-to-end performance of \sys and baseline systems. Here latency is reported as the time-per-output-token (decoding latency). We create a varying inference workload for different MoE models, and the intensity of the workload is controlled by the Request-Per-Second (RPS) by the clients. For both \sys and baseline systems, we implement the auto-batching of requests based on the maximal latency and maximal batch size. These described configurations are consistent with papers reported in vLLM and Orca~\cite{orca}. In this set of experiments, we use a single GPU on our server to create the most challenging limited resource scenario. 

Figure~\ref{fig:rps-latency} reports the end-to-end performance. For Mixtral-8x7B (the worst case for us due to its small number of experts per layer and a relatively high activation ratio), \sys can still achieve latency down to 836ms, and sustain it until the RPS is over 0.2 (see Figure~\ref{fig:rps-latency}(c)). At the same time, the GPU-Rich user consumes 8 GPUs, achieving a latency as 175ms, but can sustain it until RPS over 0.4. This indicates that \sys can save GPU resources by 4X but only compromising RPS to half, already useful for many GPU-limited users. For all other offloading-supported baselines, \sys's latency performance is close to BrainStorm and Llama.cpp but achieves over 7-8X improved RPS. For DeepSpeed-Inference and Mixtral-Offloading, their latency are even worse, mainly due to their poor prefetching and caching performance. 

For MoE models with more experts per layer and low selective activation ratios, the performance gains of \sys become more significant. For Switch and NLLB, see Figure~\ref{fig:rps-latency}(a) and (b), \sys achieves the 155ms and 531ms latency, both numbers comparable to those with the GPU-Rich. \sys can sustain this latency performance to around 80\% of the RPS by the GPU-Rich. This means significant GPU saving by \sys: achieving similar latency and RPS performance, \sys requires a single GPU while the GPU-Rich requires 8 GPUs for NLLB and 4 GPUs for Switch. Other offloading-supported systems, however, cannot provide such a promise. Benefiting from correlation analysis and accurate on-demand prefetching, BrainStorm and Mixtral-Offloading can achieve low latency but their performance quickly deteriorate with increasing RPS, almost 20X lower than \sys. DeepSpeed-Inference suffers from inaccurate prefetching and caching. As a result, it shows the worst latency and RPS performance. Llama.cpp requires custom kernels for different MoE models and it cannot run NLLB, Switch and Arctic.

For the biggest MoE model, Arctic, which has 900GB parameters (see Figure~\ref{fig:rps-latency}(d)), the GPU-Rich cannot deploy it into all the available GPUs, facing out-of-the-memory issue even budget if not an issue. In such a case, \sys becomes the only available serving system that can offer competitive inference performance with a single GPU, vastly surpassing other baseline systems. Even the GPU-Rich starts to consider  \sys (through \sys's multi-GPU support) to address its out-of-memory issue.

\begin{figure}[t]
    \centering
    \begin{minipage}{\linewidth}
        \centering
        \includegraphics[width=\linewidth]{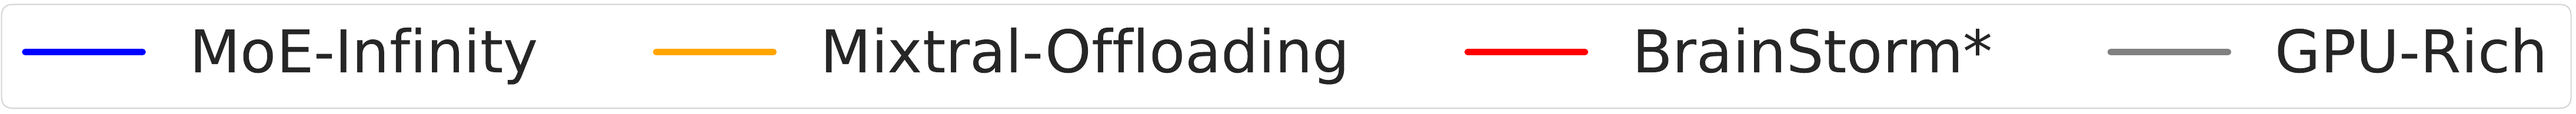}
    \end{minipage}
    \begin{minipage}{0.48\linewidth}
        \includegraphics[width=\linewidth]{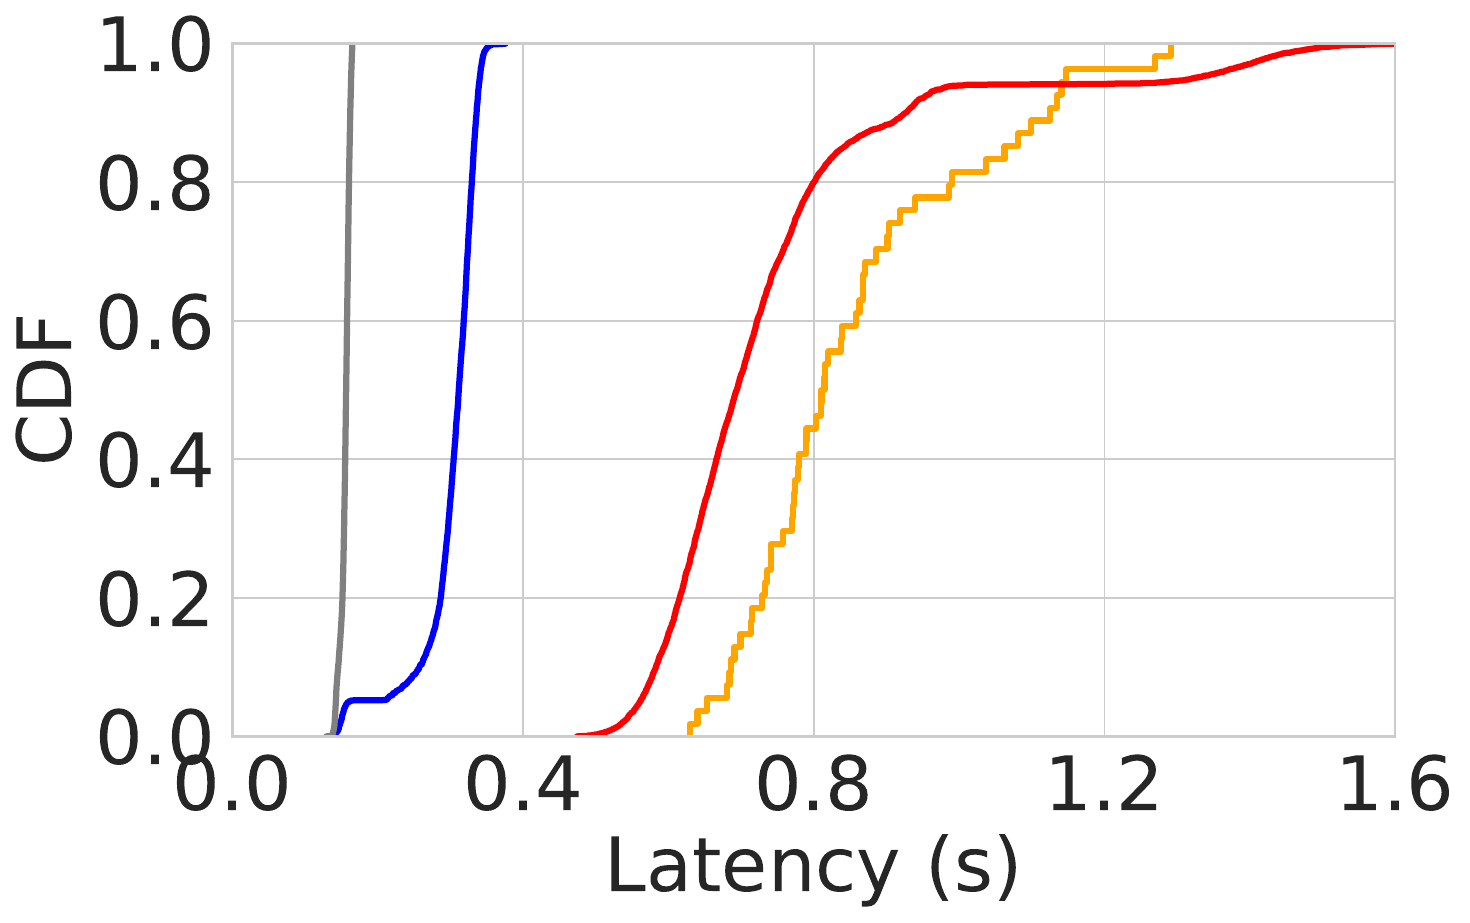}
        \caption{Switch-128x0.2B}
        % \label{fig:latency-cdf-switch}
    \end{minipage}
    \hfill
    \begin{minipage}{0.48\linewidth}
        \includegraphics[width=\linewidth]{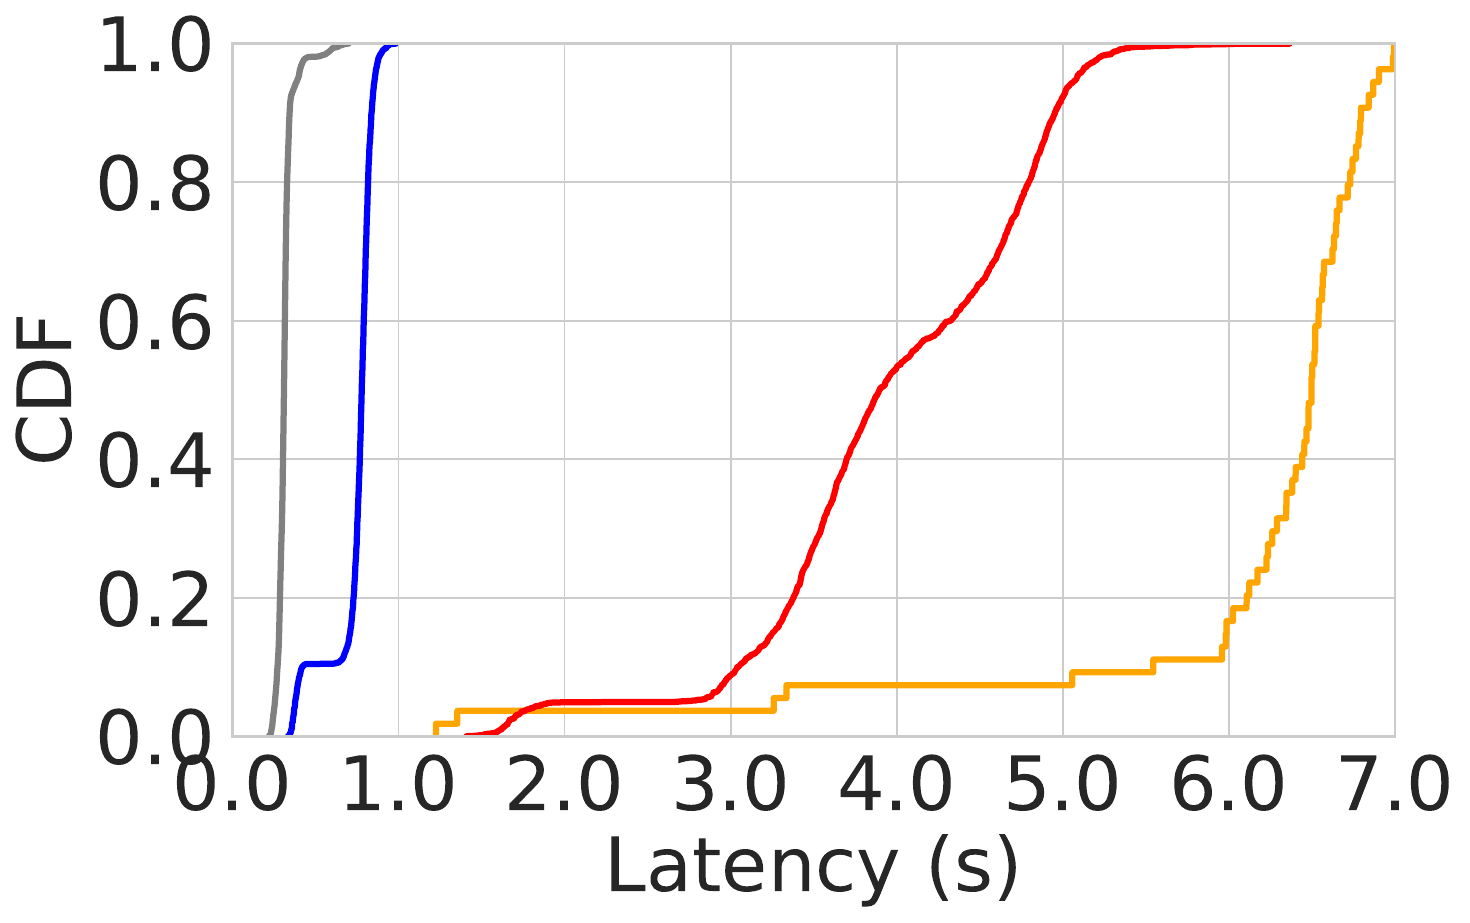}
        \caption{NLLB-128x0.4B}
        % \label{fig:latency-cdf-nllb}
    \end{minipage} 
    \caption{Tail latency.}
    \label{fig:latency-cdf}
\end{figure}

\mypar{Tail latency} We also wonder if offloading would affect tail latency, a metric that matters in serving scenarios. For this, we report the CDF graph for Switch (RPS=1.5) and NLLB (RPS=0.6) with \sys in Figure~\ref{fig:latency-cdf}. With these two RPS settings, \sys has saturated the usage of the PCIe bandwidth and the GPU. In such a case, the gap of the tail latency between \sys and the GPU-Rich is still close, similar to the averaged latency reported above. This is attributed to \sys's design in effectively handling the contention of buffer slots in the GPUs as well as the contention on the PCIe connection.

\begin{figure}[t]
    \centering
    \begin{minipage}{\linewidth}
        \centering
        \includegraphics[width=0.6\linewidth]{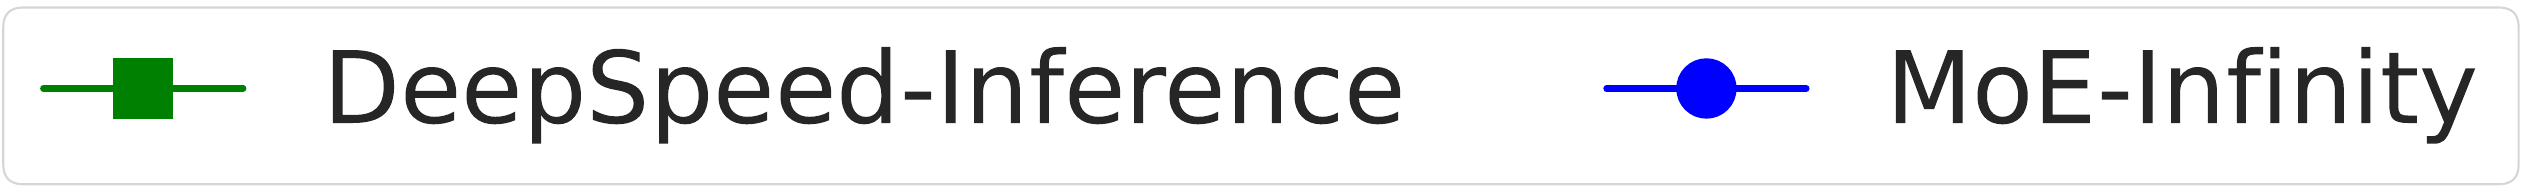}
    \end{minipage}
    \begin{minipage}{0.48\linewidth}
        \includegraphics[width=\linewidth]{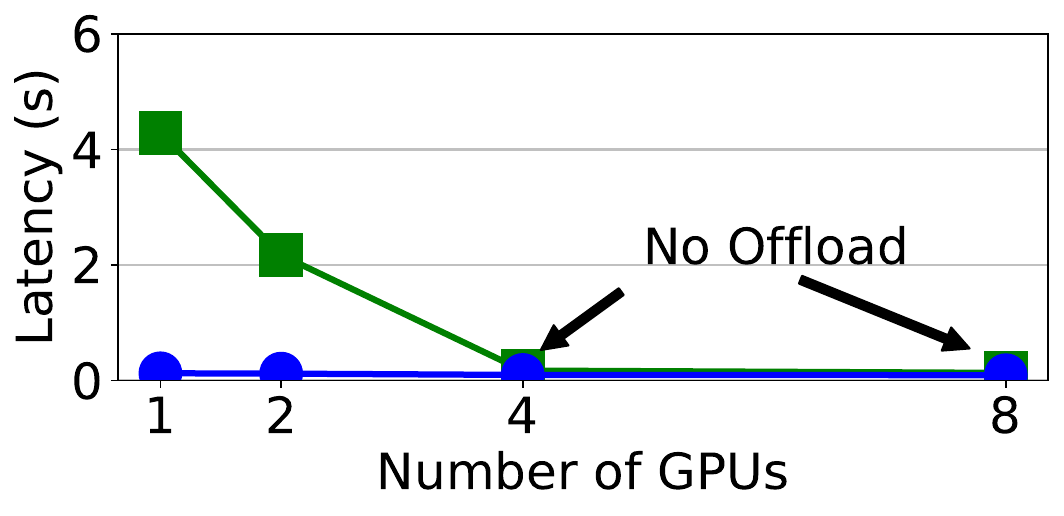}
        % \caption{Switch-128x0.2B}
        \label{fig:resource-efficiency-switch}
    \end{minipage}
    \hfill
    \begin{minipage}{0.48\linewidth} 
        \includegraphics[width=\linewidth]{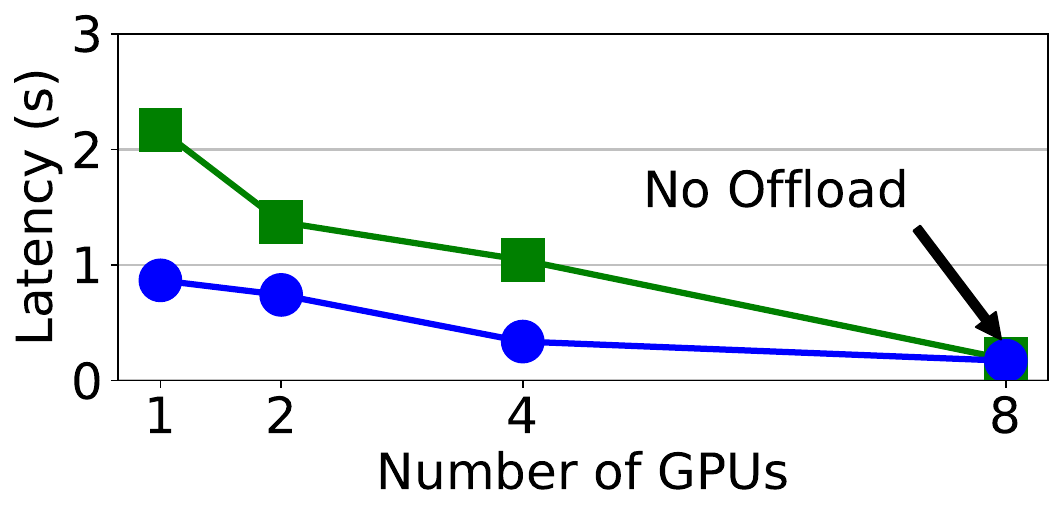}
        % \caption{Mixtral-8x7B}
        \label{fig:resource-efficiency-mixtral}
    \end{minipage}
    \hfill
    \vspace{-0.15in}
    \begin{minipage}{\linewidth}
        \centering
        \includegraphics[trim={0 4in 0 0},clip,width=\linewidth]{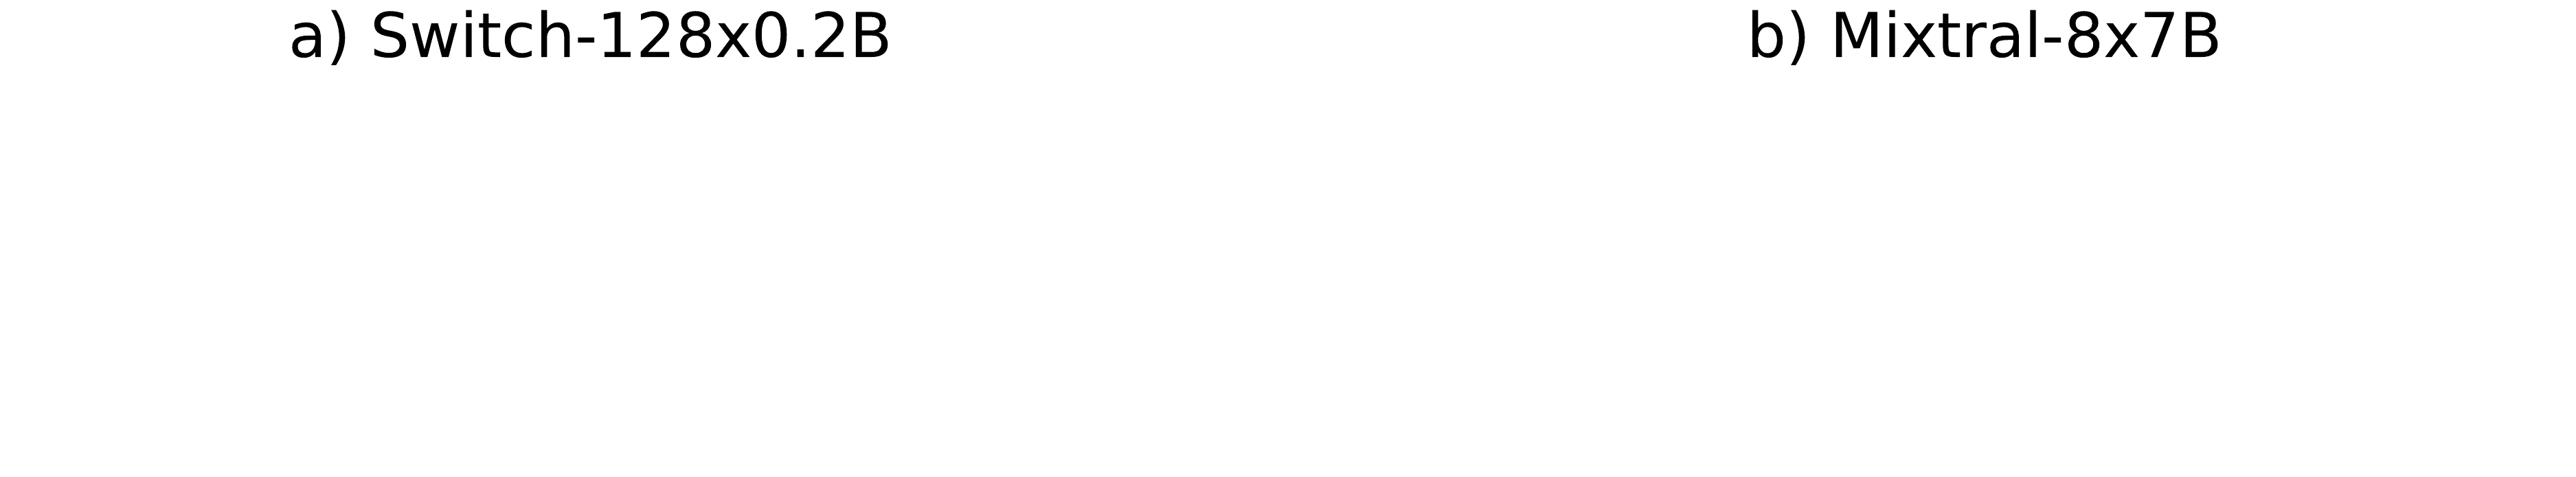}
    \end{minipage}
    \caption{GPU memory vs Host memory.}
    % \vspace{-0.1in}
    \label{fig:resource-efficiency}
\end{figure}

\mypar{GPU memory vs. host memory} The user of \sys often wonders what is best the ratio for GPU memory and host memory. We answer this question by scaling the deployment of \sys from 1 GPU to 8 GPUs, increasing the provision of GPU memory and compute resources while keeping the size of host memory (1TB) constant. Figure~\ref{fig:resource-efficiency} reports the results. Here we only include DeepSpeed-Inference since it is the only baseline library that can effectively scale its performance in a multi-GPU deployment. Benefiting from the relatively small size of the model, \sys can already achieve the best latency performance with a single GPU, whereas DeepSpeed-Inference needs 4 GPUs to achieve the best possible latency, 4X more than \sys.

For bigger NLLB-MoE, \sys would require more PCIe bandwidth and GPU memory. In such a case, even though it can still achieve below 1 second performance with a single GPU, its best latency performance would require 4 GPUs. At the same time, DeepSpeed-Inference would require all 8 GPUs to make it latency performance below 1 second.

\begin{figure}[t]
    \centering
    \begin{minipage}{\linewidth}
        \centering
        \includegraphics[width=.85\linewidth]{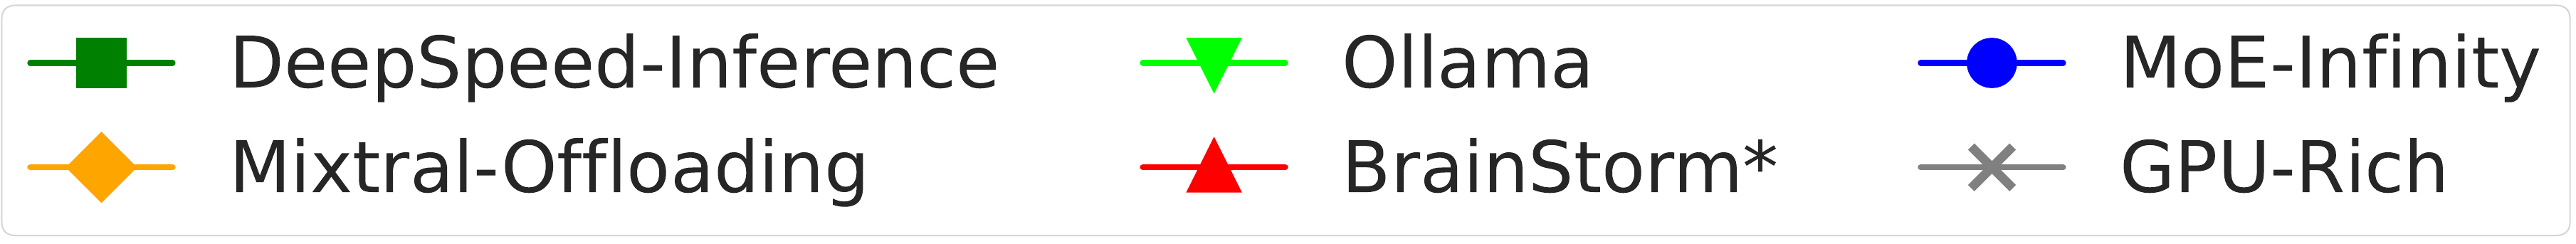}
    \end{minipage}
    \begin{minipage}{0.48\linewidth}
        \includegraphics[width=\linewidth]{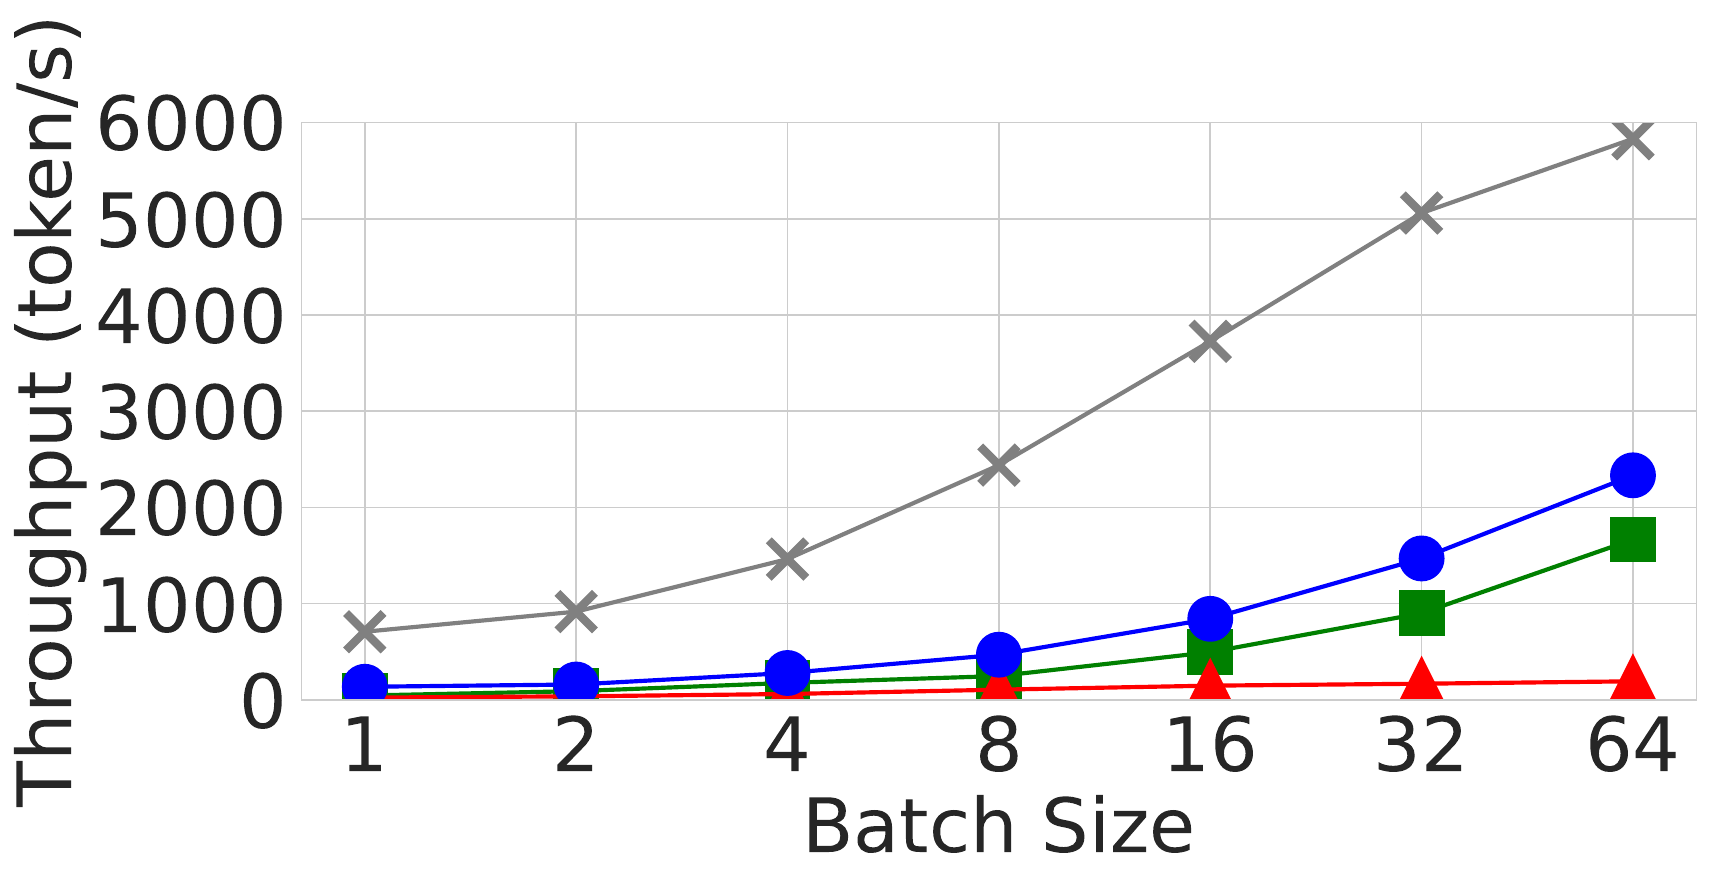}
        % \caption{NLLB-128x0.4B}
        \label{fig:prefilling-throughput-nllb}
    \end{minipage}
    \hfill
    \begin{minipage}{0.48\linewidth} 
        \includegraphics[width=\linewidth]{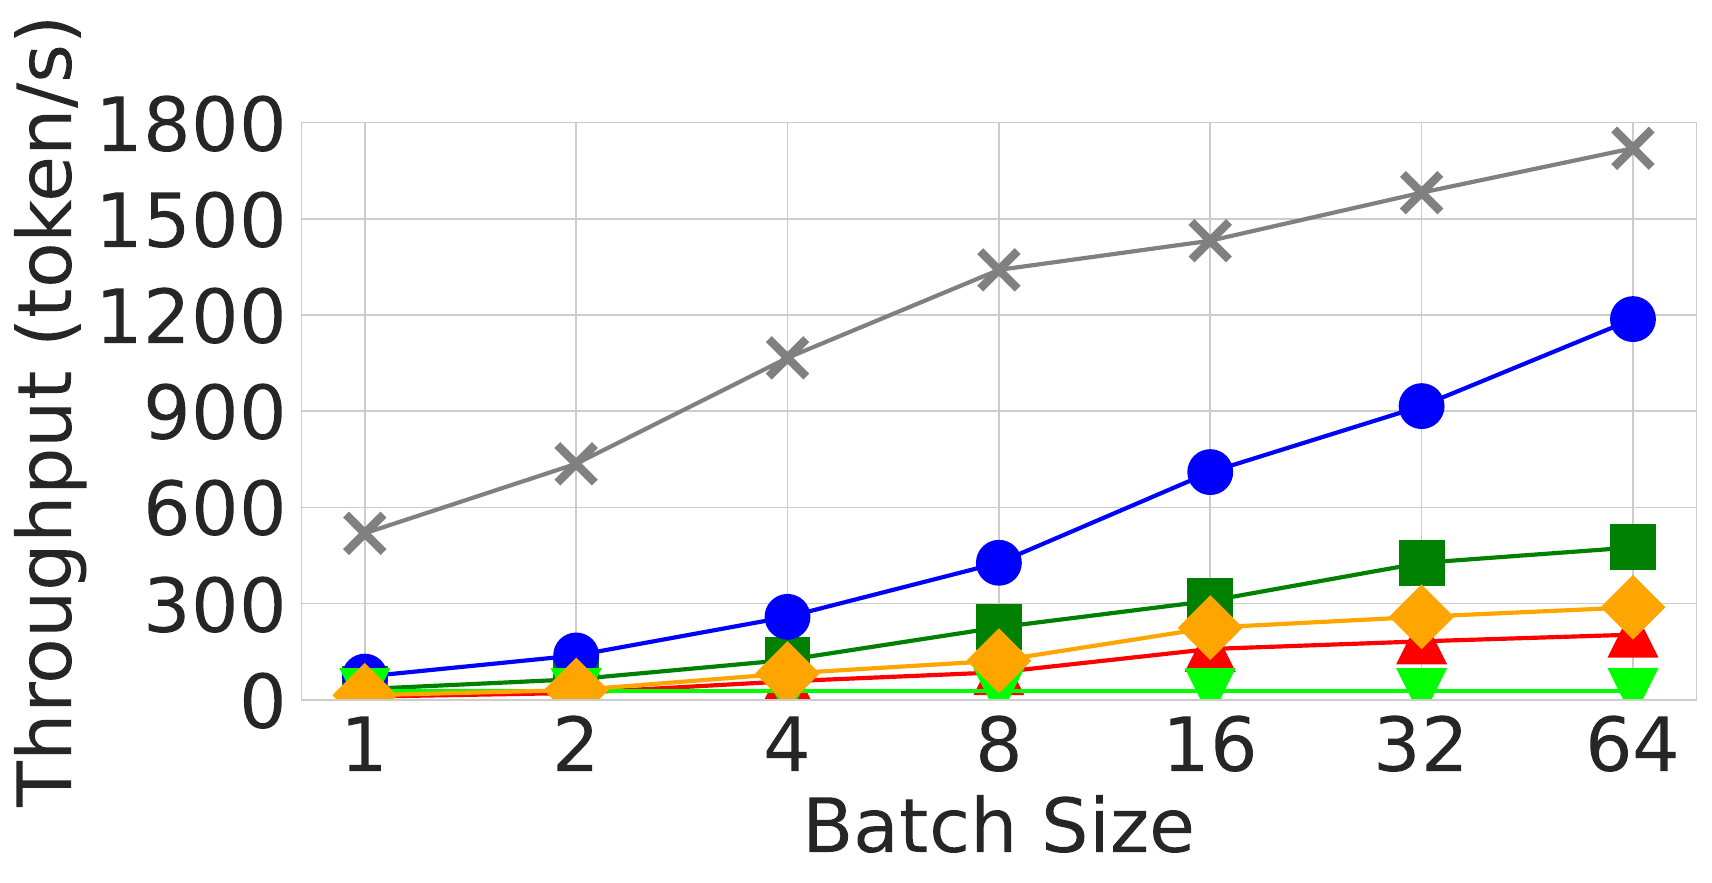}
        % \caption{Mixtral-8x7B}
        \label{fig:prefilling-throughput-mixtral}
    \end{minipage}
    \hfill
    \vspace{-0.15in}
    \begin{minipage}{\linewidth}
        \centering
        \includegraphics[trim={0 4in 0 0},clip,width=\linewidth]{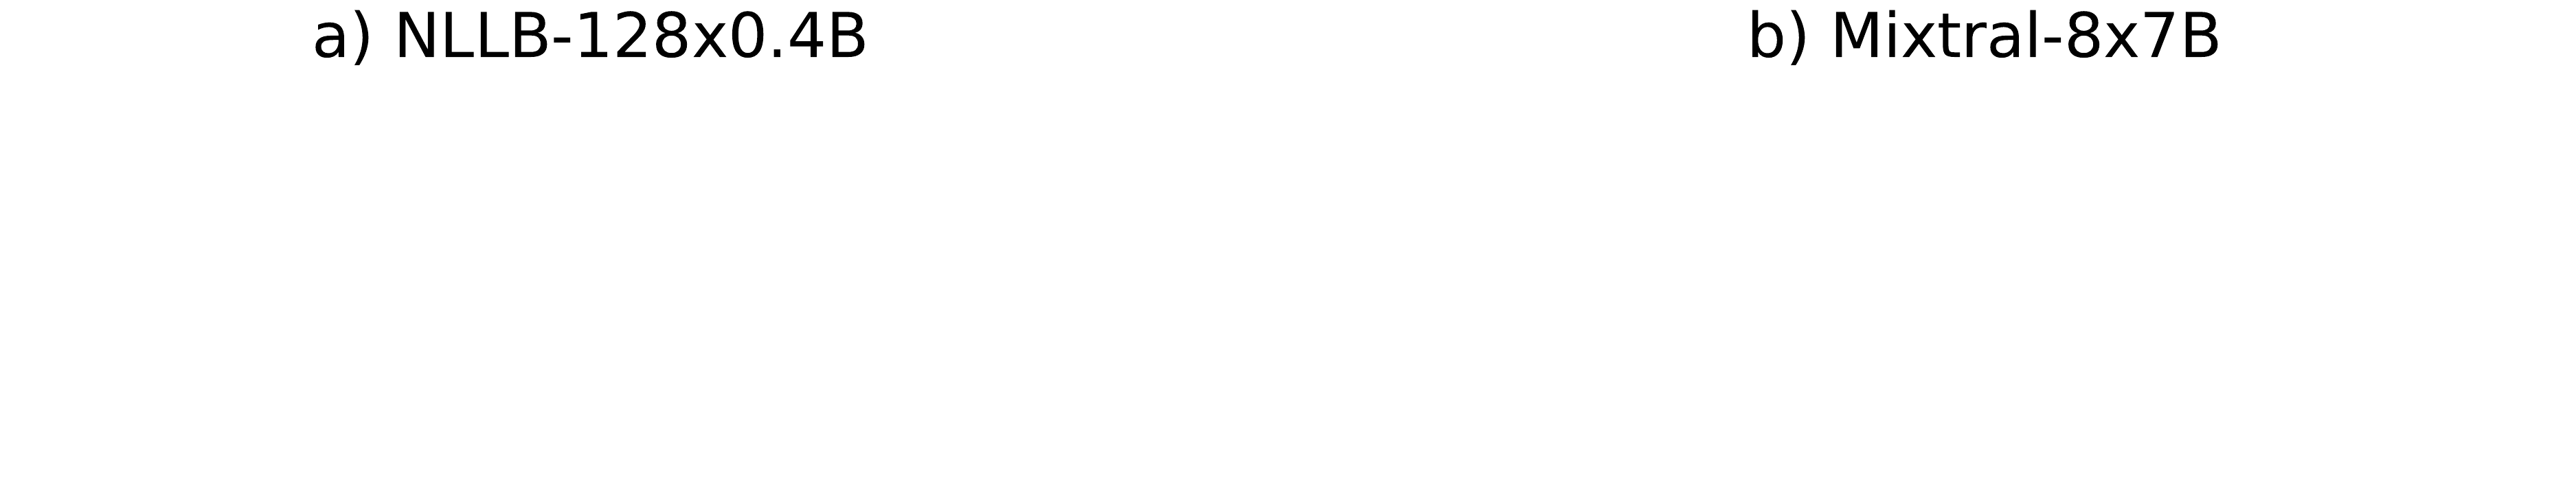}
    \end{minipage}
    \caption{Prefill Performance.}
    % \vspace{-0.1in}
    \label{fig:prefilling-throughput}
\end{figure}

\mypar{Cost saving through sharing servers} We demonstrate how \sys enables cost saving when serving MoE models for the GPU poor. By considering multiple MoE models with architectures similar to NLLB, \sys allows these models to share a single 8-GPU server. This is achieved by deploying multiple \sys instances on the server and evenly partitioning the GPUs and host memory among them. Previously, users had to invest in expensive, dedicated 8-GPU servers; without such resources, they faced memory shortages or were forced to resort to slower offloading techniques that compromised latency and throughput. Table~\ref{tab:cost-efficient-nllb} reports the results.
Instead of using 4 AWS-A10G instance with 8x24GB GPU memory each, we deploy each model with 2 GPUs and enable offloading with \sys. Such deployment save 4x cost while only have 130ms latency and 4 RPS degradation. For the Switch model, we observed similar degrees of cost saving through sharing servers, and we omit their results due to the page limit.

\begin{table}[t]
    \centering
    \caption{Effective sharing of servers to save GPU cost}
    \begin{tabular}{cccccc}
    \hline
        System  & Config. & RPS & Latency (s) & Cost (\$/hr) \\
    \hline
        \sys & 4 models / server & 9 & 0.379 & 16\\
        GPU-Rich & 1 model / server & 13.2  & 0.249 & 64\\
    \hline
    \end{tabular}
    \label{tab:cost-efficient-nllb}
\end{table}

\mypar{Prefill performance} So far, we have been focusing on reporting decoding performance, consistent with that reported by other papers on LLM serving. For offloading to be applicable in serving scenarios, users might also question whether it significantly slows down prefilling. To address this, we report prefill performance in terms of token throughput, the typical metric for this phase since it is throughput-oriented. Figure~\ref{fig:prefilling-throughput} presents the results. 
As we can see, 
% for large MoE models with many experts per layers, \sys can still achieve high throughput. This is because for many instances in the prefill phase, the low activation ratios and group activation patterns still emerge, facilitating prefetching and caching. 
among offloading-support systems, \sys achieves the best performance, benefiting from its better prefetching and caching designs. For Mixtral, the worst case for \sys, the prefill throughput is 1187 tokens per second for a batch size of 64. For NLLB, the prefill throughput reaches 2333 tokens per second for the same batch size. The result shows that even with high activation ratios, \sys can still effectively overlap prefetching and inference, and its caching strategy still shows benefits over existing GPU caching strategies (as in Llama.cpp and Mixtral-Offloading).

% \section{Breakdowns for Prefetching and Caching}
% \label{sec:appendix-breakdowns}

\subsection{\sys Prefetching Strategy}
\label{sec:eval-expert-prefetching}

\begin{table}[t]
    \centering
    \begin{tabular}{|c|c|c|c|c|c|}
    \hline
        Model   & Dependency&Model-tracing&On-demand  & Ours \\
    \hline
        Switch  &    230\%   &  51\%     & 100\%      & 12\%  \\
        NLLB    &    147\%   &  71\%     & 100\%      & 31\%  \\
        Arctic  &    195\%   &  63\%     & 100\%       & 43\%  \\
        Mixtral &    147\%   &  91\%     & 100\%       & 37\%  \\
    \hline
    \end{tabular}
     \caption{Normalized GPU blocking time.}
    \label{tab:gpu-blocking-time}
\end{table}

\begin{table}[t]
    \centering
    \begin{tabular}{|c|c|c|c|c|c|}
    \hline
        Model   & Dependency&Model-tracing&On-demand  & Ours \\
    \hline
        Switch  & 239\%      &   204\%    & 100\%       &  168\% \\
        NLLB    & 148\%      &   127\%    & 100\%       &  126\% \\
        Arctic  & 183\%      &   186\%    & 100\%       &  187\% \\
        Mixtral & 143\%      &   101\%    & 100\%       &  143\% \\
    \hline
    \end{tabular}
    \caption{Normalized bandwidth usage.}
    \label{tab:bandwidth-usage}
\end{table}

We first assess the prefetching strategy in \sys. We consider the following baseline strategies:
(i)~\emph{Dependency-based prefetching strategy}, used in DeepSpeed-Inference, which constructs a computational graph for an MoE model. Since all experts in the next layer exhibit computational dependency on the currently executed expert, all next-layer experts are potentially activated and thus prefetched;
(ii)~\emph{Model-tracing-based prefetching strategy}, used in BrainStorm, which counts operator usages across the entire lifetime of the serving system and prefetches most used operators in the next MoE layer; and
(iii)~\emph{On-demand prefetching strategy}, used in Mixtral-Offloading and Ollama, which initiates prefetching experts only after the router in the current layer has dispatched its tokens, achieving optimal bandwidth usage but delaying prefetching onset.

To assess prefetching performance independently, we disable the caching of the experts in all systems (\ie experts are released from the buffer immediately after being used). Here we measure two important metrics that reflect the prefetching performance: GPU blocking time and prefetching bandwidth usage:

\mypar{GPU blocking time} An effective prefetching strategy should begin prefetching early to ensure experts are available when needed, minimizing GPU blocking time. The evaluation of prefetching strategies is presented in Table~\ref{tab:gpu-blocking-time}. On-demand fetching latencies for experts are 1ms, 2.5ms, 7ms, and 10ms for Switch to Mixtral, respectively, mirroring single expert inference latencies. Dependency-based prefetching performs worse than on-demand due to I/O contention from excessive traffic. \sys achieves a latency reduction of 20x on Switch and 4x on other models through sequential and selective prefetching. Model-tracing-based prefetching is effective for skewed expert access patterns but less so for uniform patterns in Mixtral. \sys, utilizing the EAM for prediction, achieves a 1.5-2.5x latency reduction by identifying per-request patterns.
% \todo{describe the results in absolute values, show performance improvement ratios, explain why we are better. Provide insights why baseline fails. Remember don't repeat the same, lengthy argument in previous sections but link/cite them here. We need insights from the data.}

\mypar{Bandwidth usage} A good prefetching strategy shall also minimize its bandwidth usage, minimizing the number of prefetched experts actually not used by the GPUs. We report bandwidth usage in Table~\ref{tab:bandwidth-usage}. 
On-demand fetching represents the minimal bandwidth usage as it is exact.
Dependency and model-tracing strategy can use up to 2x the bandwidth in Switch and Arctic, as they provide incorrect prefetching, and later falls back to on-demand.
Both the model-tracing strategy and our strategy can use cancels to reduce traffic, prominent in the case of Mixtral. 
\sys uses slightly more traffic, however, 56\% of the excessive ones can be overlapped with inference, resulting in less overhead than baselines which fall back to on-demand fetching.
Among all traffic 68\% for Arctic and 81\% for NLLB are hit in GPU.

% \todo{Succinctly, carefully describe the results. Provide insight discussion supported by your experimental results. Don't repeat the same arguments in Section 4 and 5. Here, focus on data, data, data to support your insights.}

\begin{table}[t]
    \centering
    \begin{tabular}{|l|c|c|c|}
    \hline
        Designs             & Bandwidth usage   & Blocking time \\
    \hline
        Vanilla prefetching &    100\%            & 100\%       \\
        + Request-level tracing        &    56\%           & 55\%      \\
        + Multi-layer       &    73\%           & 39\%       \\
        + Layer-proximity   &    68\%           & 32\%      \\
    \hline
    \end{tabular}
    \caption{Performance breakdown of prefetching designs.}
    \label{tab:prefetch-breakdown}
\end{table}

\mypar{Performance breakdown} We also want to understand how the multiple new design intuitions (detailed in Section~\ref{sec:expert-prefetching-strategy}) independently contribute to the improved GPU blocking time and bandwidth usage. For this, we provide a performance breakdown shown in Table~\ref{tab:prefetch-breakdown}. 
Vanilla provides fixed size dependency prefetch.
Request-level tracing tends to be the biggest factor in improving bandwidth usage and the GPU blocking time, improving them 43\% and 45\%, respectively. Turning on multi-layer prefetching increases prefetching traffic, as expected; however, it greatly reduces GPU blocking time by 16\%. Finally, the layer proximity design saves the bandwidth usage by 5\%, as we can more actively cancel unnecessary prefetching of experts far from the current layer. By benefiting closer experts, it reduces blocking time by 7\%.
% \todo{briefly describe the results shall be okay here since the reviewer shall have understand why these designs work previously. Highlight which one contributes the most. Maybe EAM? Also, may different metrics have different biggest contributors? If so, this is an interesting insight and we shall highlight this.}
