# Supplementary material for: MoE-Infinity: Efficient MoE Inference on Personal Machines with Sparsity-Aware Expert Cache
Source: arXiv:2401.14361 source file (2025-03-12)
Supplement: Supplementary file 2 [file appendix-observations.tex]

\section{Expert Activation Awareness}\label{sec:appendix-observations}

\begin{figure}[t]
    \centering
    \begin{minipage}{0.48\linewidth}
        \includegraphics[width=\linewidth,trim={0cm 0.5cm 0cm 2cm},clip]{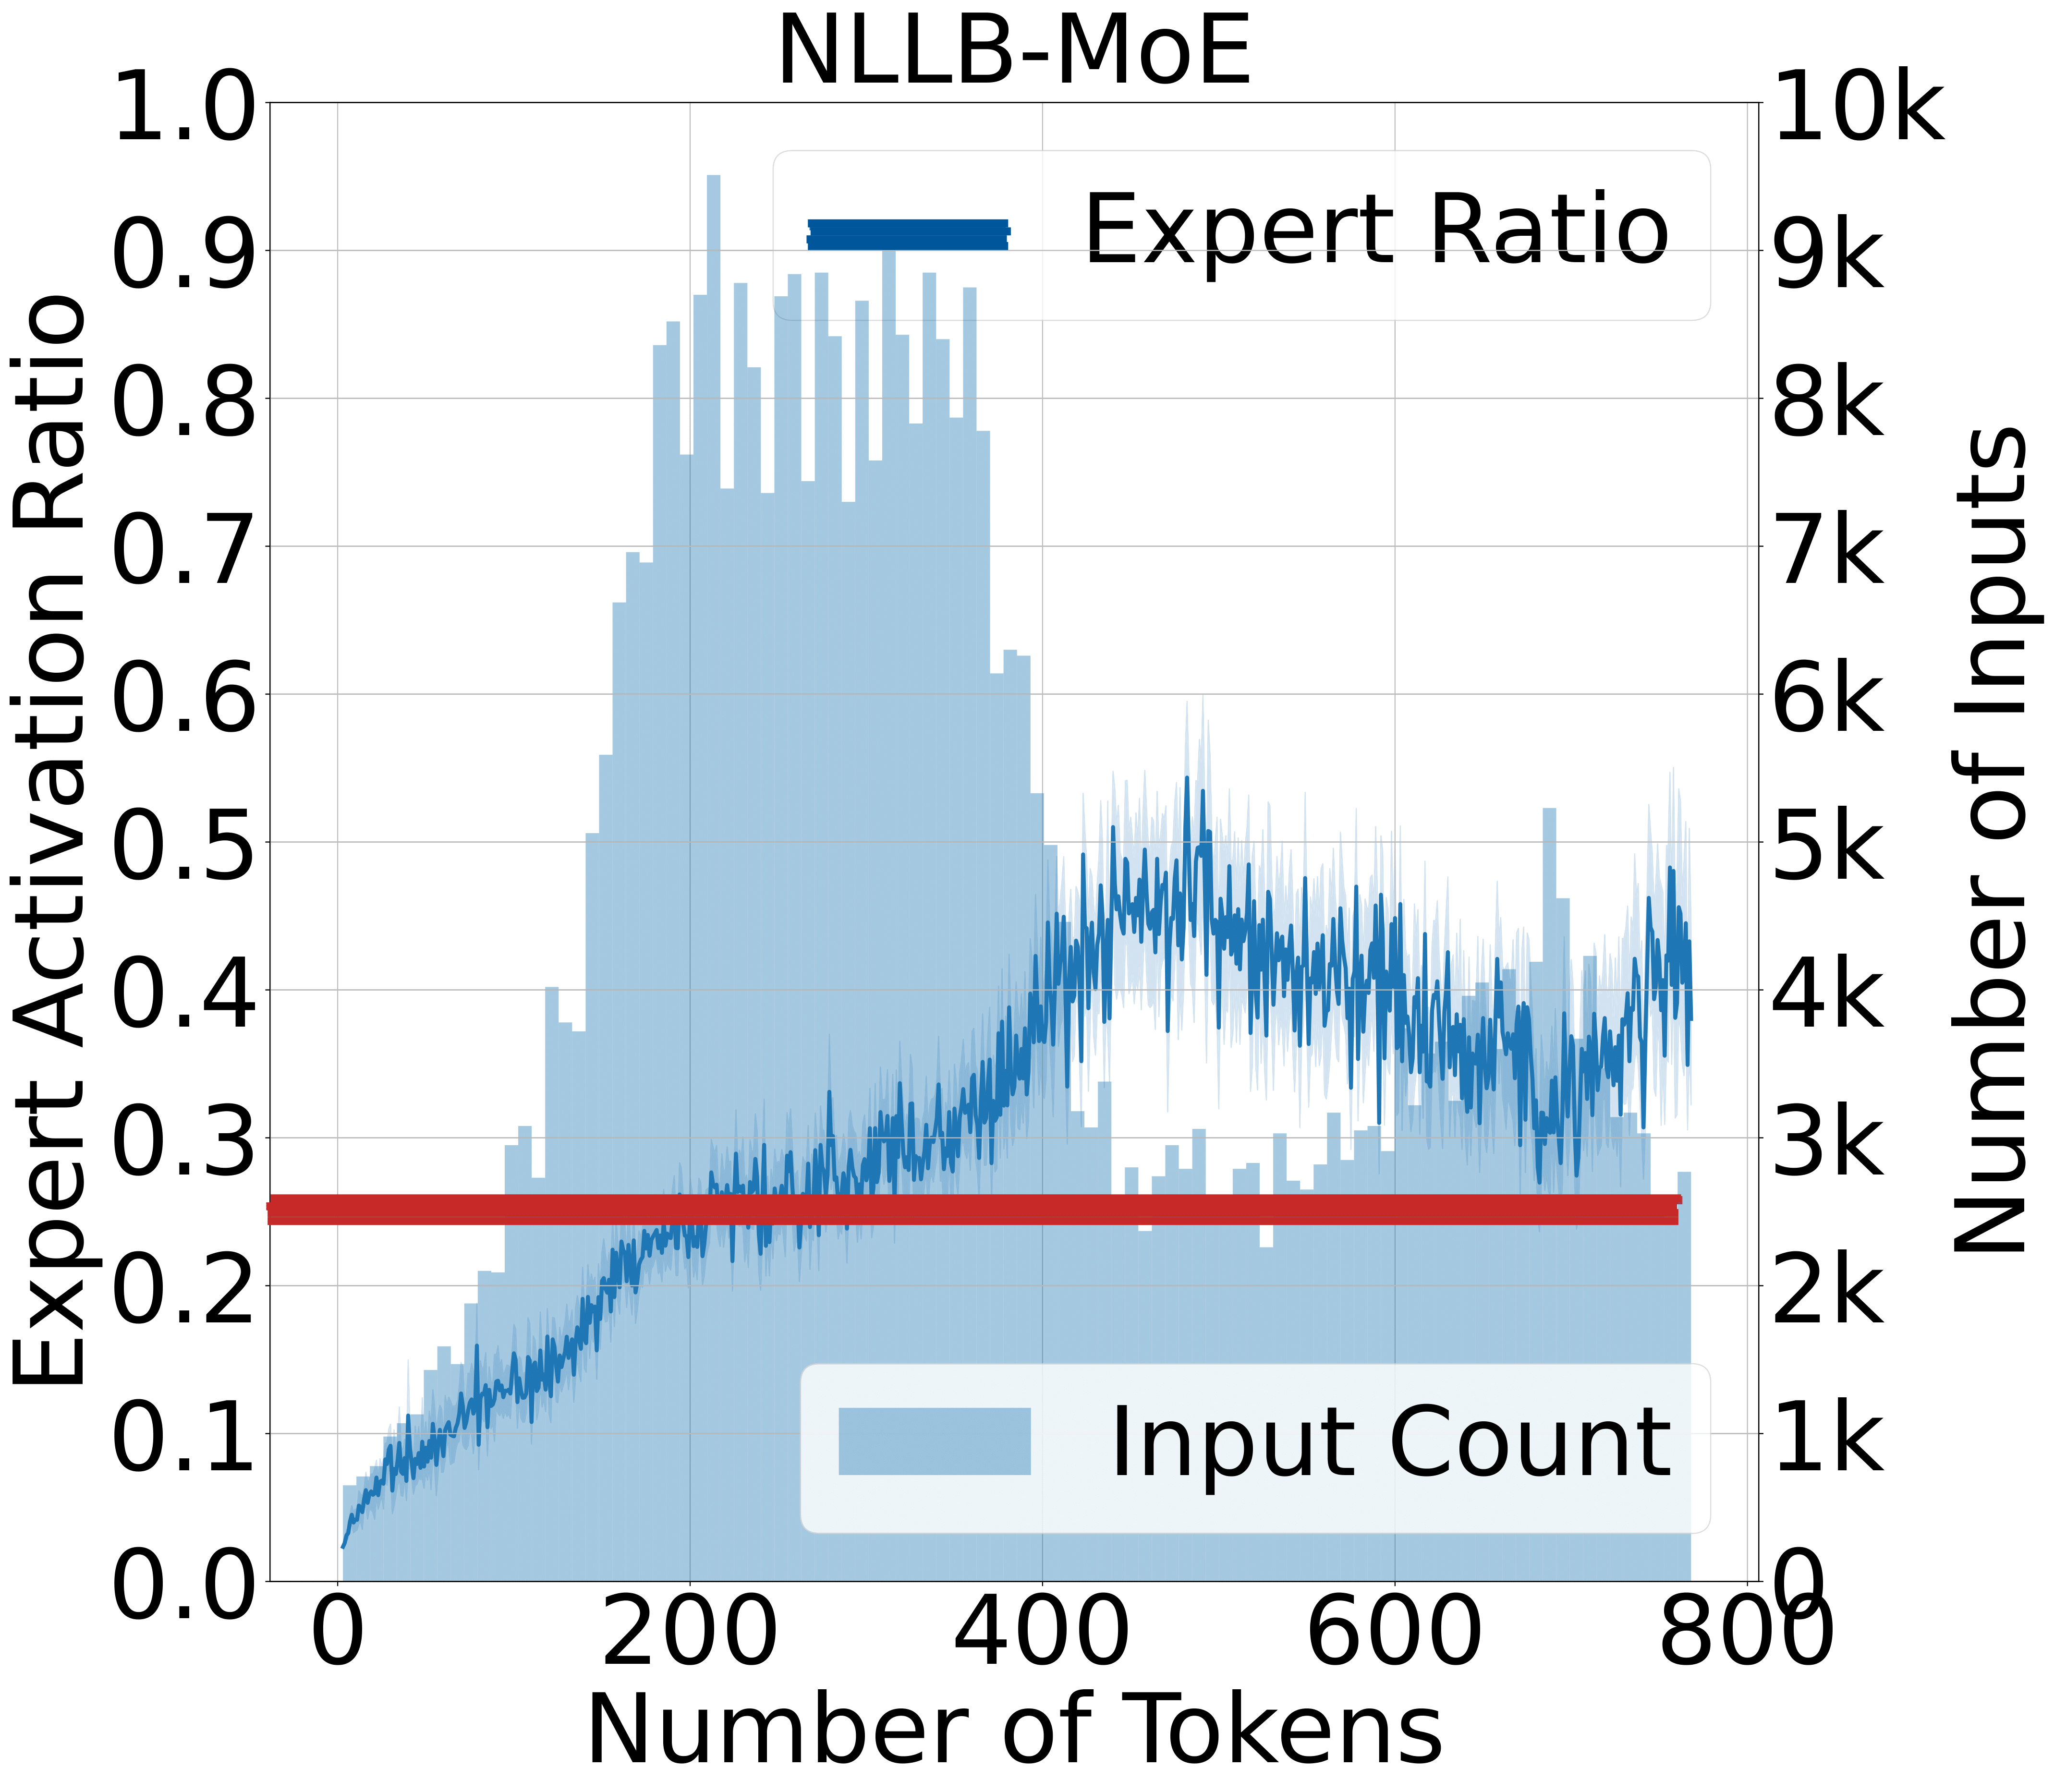}
        % \includegraphics[width=\linewidth]{figures/illustration/expert_ratio_nllb.pdf}
        % \caption{NLLB-128x0.4B}
        \label{fig:prefilling-sparsity-nllb}
    \end{minipage}
    \begin{minipage}{0.48\linewidth}
        \includegraphics[width=\linewidth,trim={0cm 0.5cm 0cm 2cm},clip]{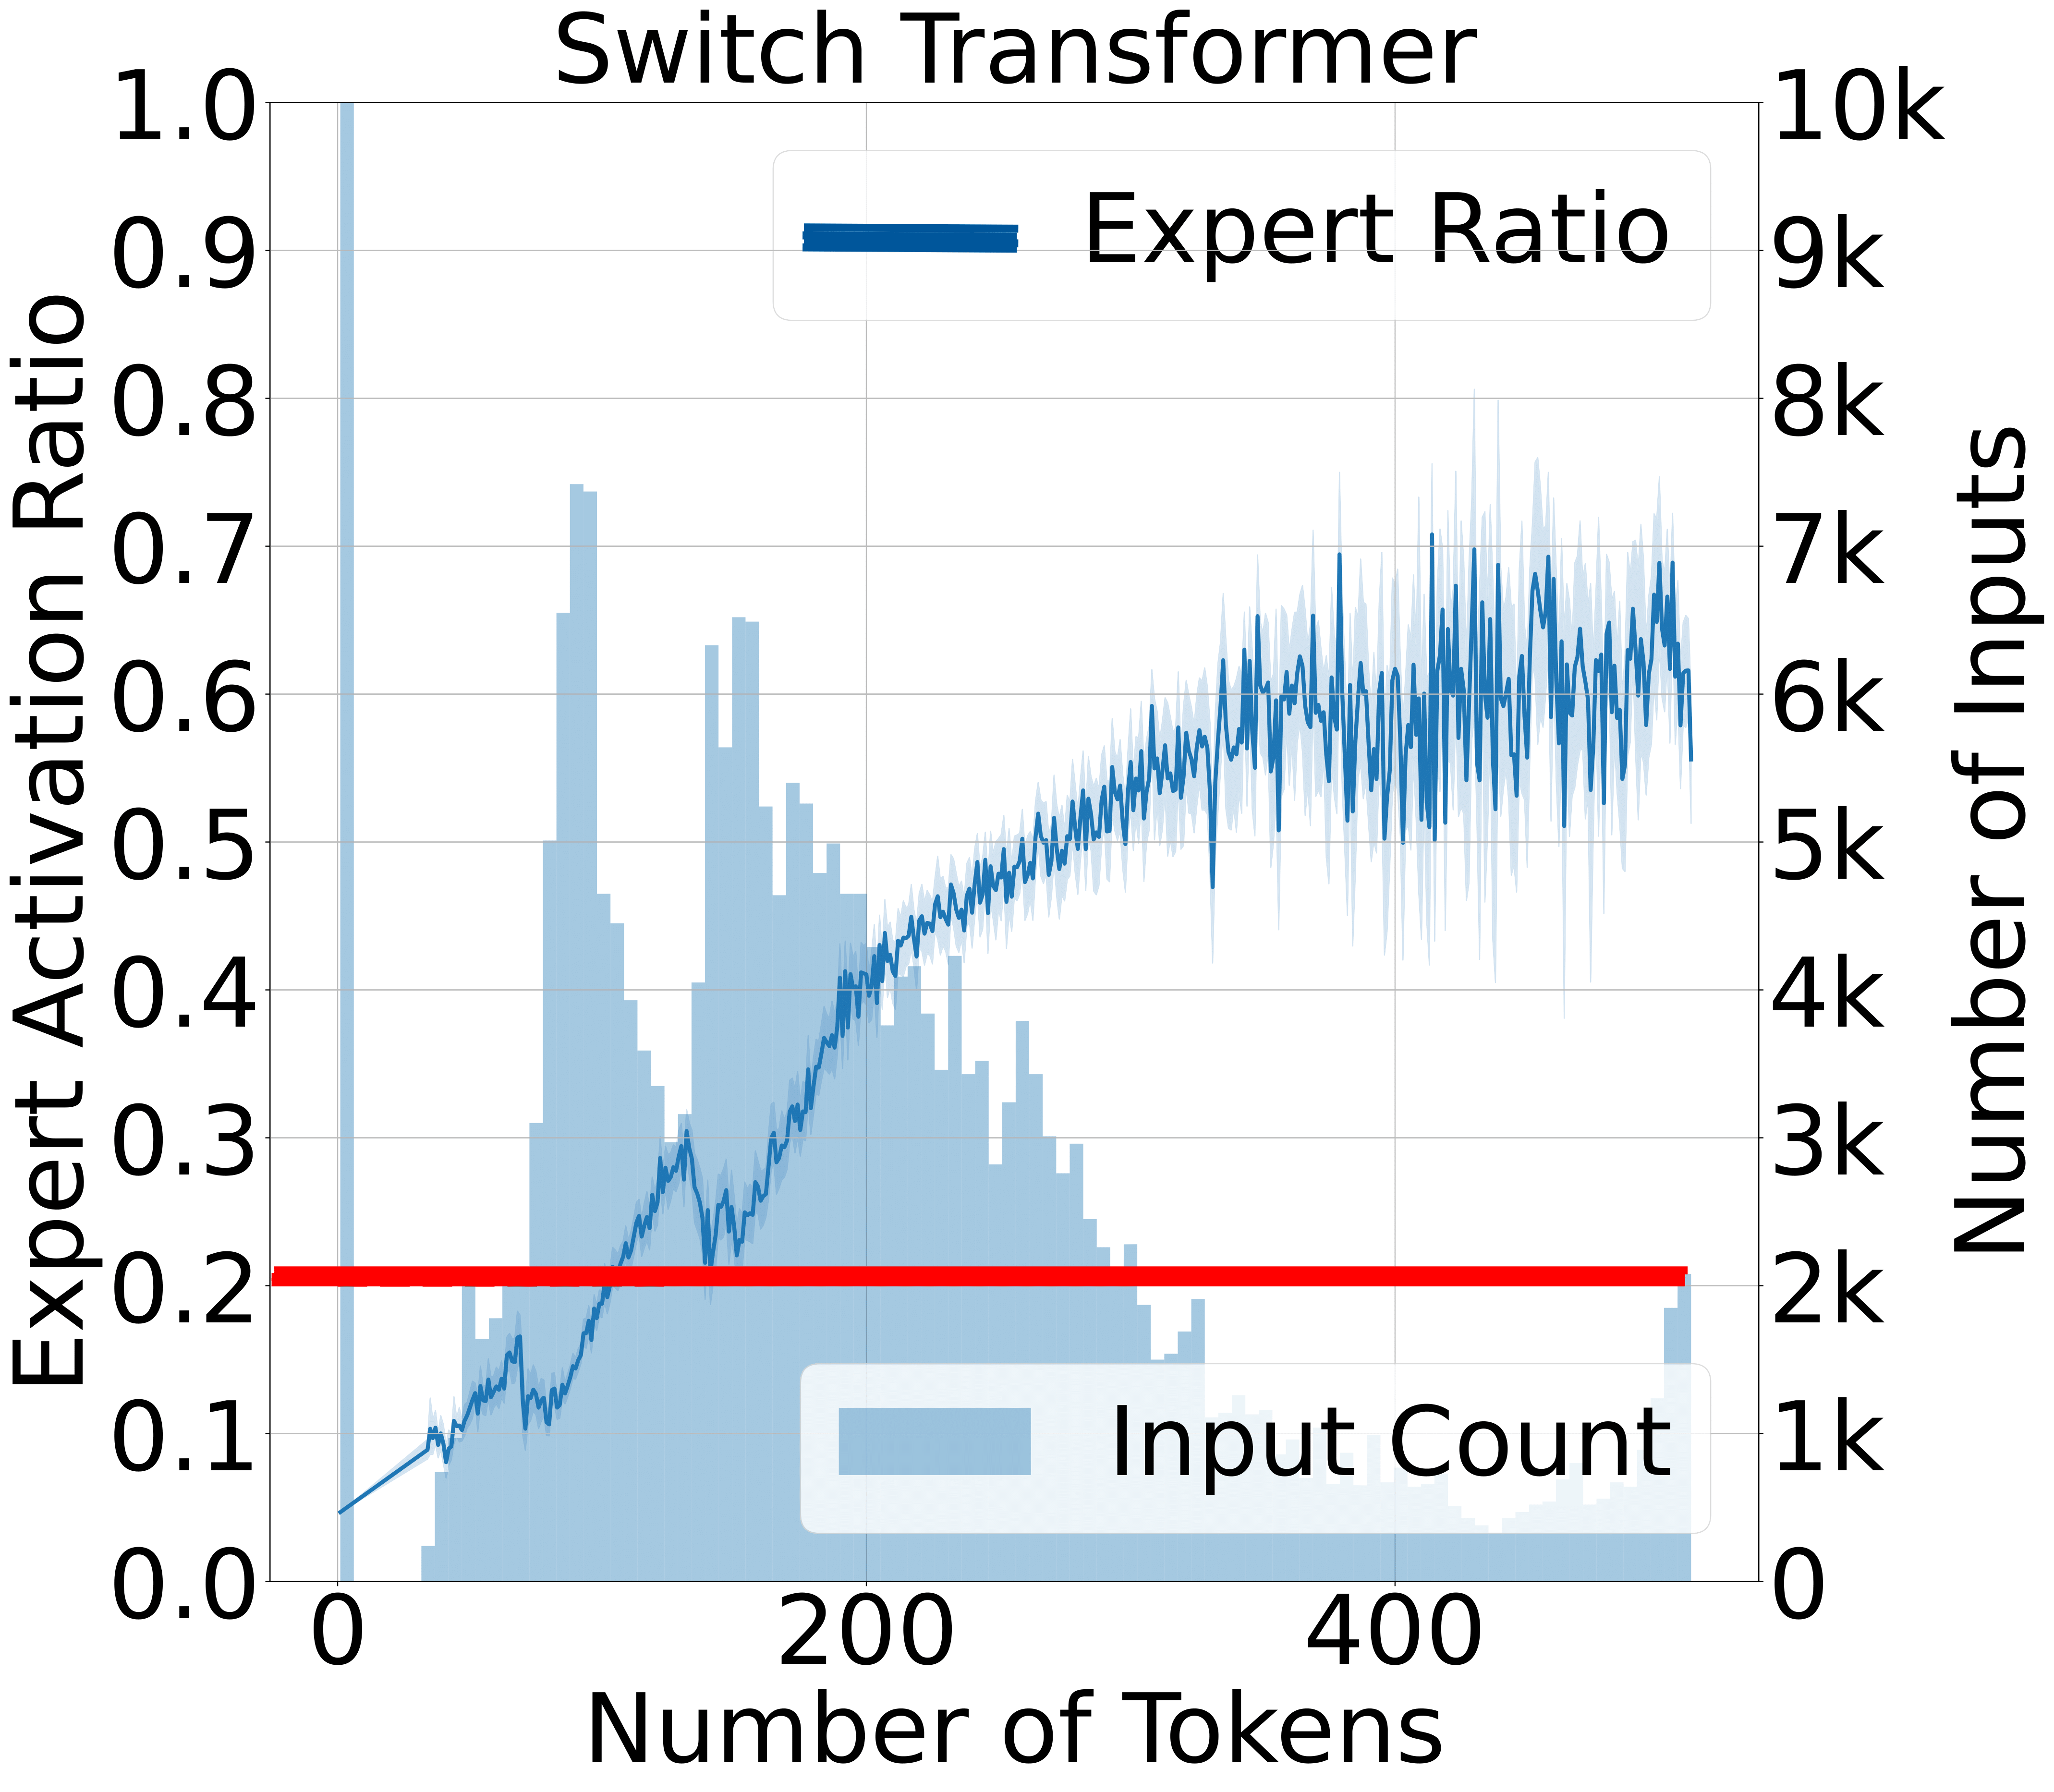}
        % \includegraphics[width=\linewidth]{figures/illustration/sequence_length_nllb-moe-54b.pdf}
        % \caption{Switch-128x0.2B}
        \label{fig:prefilling-sparsity-switch}
    \end{minipage}
    \hfill
    \vspace{-0.15in}
    \begin{minipage}{\linewidth}
        \centering
        \includegraphics[trim={0 4in 0 0},clip,width=\linewidth]{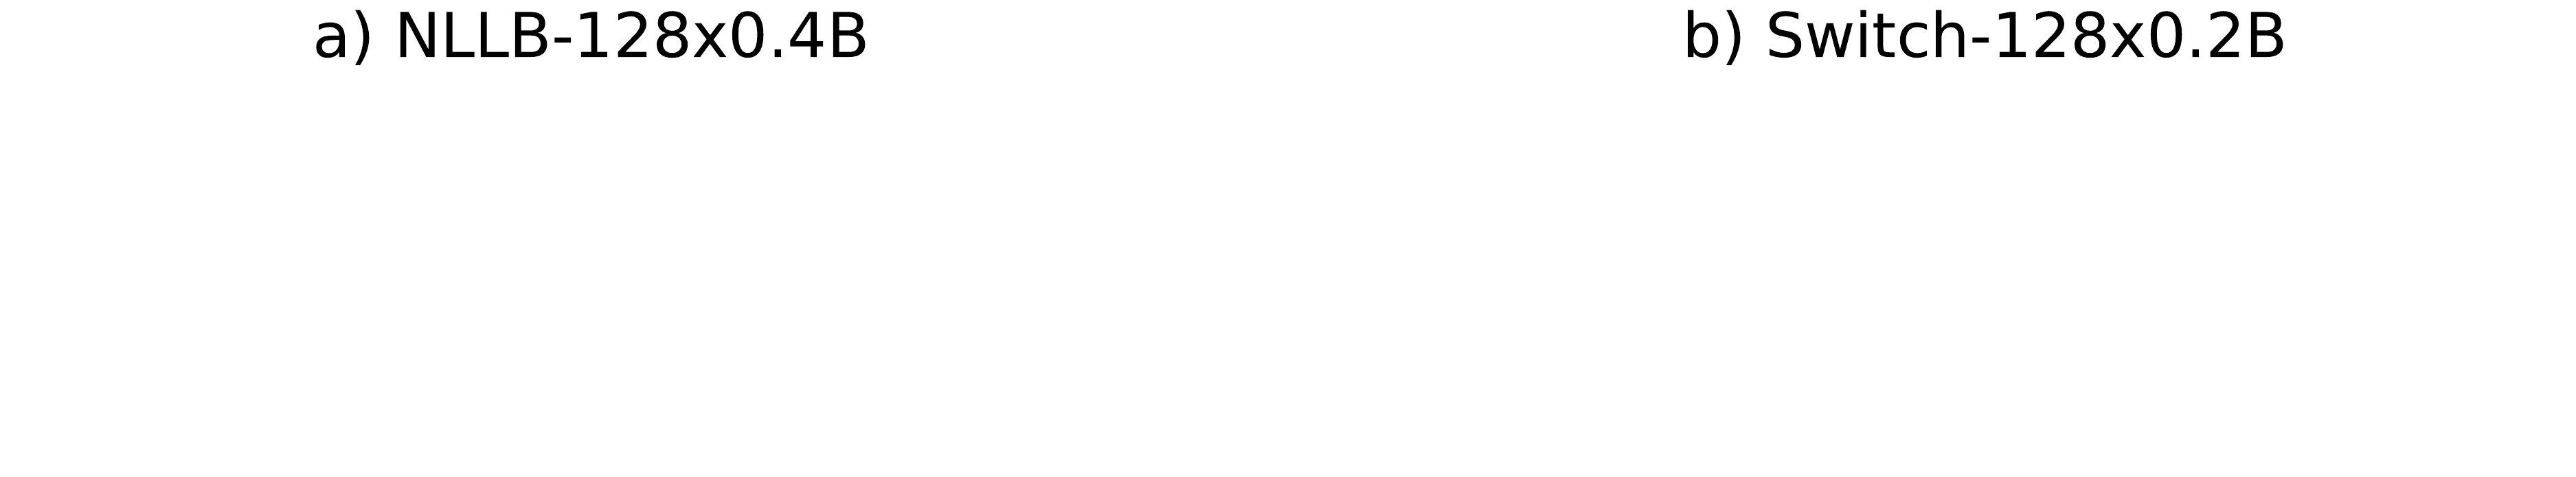}
    \end{minipage}
    \caption{Expert activation over sequence length in prefilling. The left y-axis shows the expert activation ratio by prompt length (x-axis), while the right y-axis counts prompts by length. The horizontal red line marks the average prompt length activation ratio, using BIGBench, FLAN, and MMLU.}
    \label{fig:prefilling-sparsity}
\end{figure}

\mypar{(1)~Highly selective activations}
Selective activation during the prefilling phase is evident in BIGBench and FLAN datasets, with 60\% of prompts under 200 tokens, leading to low activation ratios in models like Switch and NLLB (Figure~\ref{fig:prefilling-sparsity}). NLLB averages 26\% expert activation, increasing to 47\% for 756-token prompt (Figure~\ref{fig:prefilling-sparsity} (a)). Switch shows a lower average of 21\% (Figure~\ref{fig:prefilling-sparsity} (b)). Short prompts are more common, impacting activation trends. Unlike others, Mixtral, with eight experts per layer, often activates all experts during prefilling, underscoring its higher cost in deployment.
